# Supplementary material for: A look under the hood of the Interactive Deep Learning Enterprise (No-IDLE)
Source: arXiv:2406.19054 source file (2024-06-27)
Supplement: Supplementary file 1 [file appendix.tex]

\section{Appendix (Optional)}
